# Supplementary material for: Gaussian Process Regression for Absorption Spectra Analysis of Molecular Dimers
Source: arXiv:2112.07590 ancillary file (2021-12-15)
Supplement: Supplementary file 1 [file Supp_Mat.pdf]

# – Supplementary Material –

## Gaussian Process Regression for Absorption Spectra Analysis of Molecular Dimers

Farhad Taher-Ghahramani,<sup>1,\*</sup> Fulu Zheng,<sup>2,†</sup> and Alexander Eisfeld<sup>1,‡</sup>

<sup>1</sup>*Max Planck Institute for the Physics of Complex Systems, Nöthnitzer Str 38, Dresden, Germany*

<sup>2</sup>*Bremen Center for Computational Materials Science,  
University of Bremen, Am Fallturm 1, 28359 Bremen, Germany*

In this Supplementary Material we provide additional details on the following items:

- SI. Details of the HOPS method used for the propagation.
- SII. Details of the M-LOOP package used for the GPR.
- SIII. Exacted cost-landscapes, difference to estimated ones, and estimated uncertainty for the experiments discussed in the main text.
- SIV. Estimating the angle  $\alpha$  from the molecular structures for the experiments discussed in the main text.
- S V. Estimated cost-landscapes, exact cost-landscapes, their difference, and estimated uncertainty for two additional experiments.

### S I. DETAILS ON THE HOPS CALCULATIONS

We used the HOPS method to numerically calculate the absorption spectrum of the monomer and the dimers [1, 2]. Within the HOPS method, the correlation functions  $C_{nm}(t)$  in Eq. (8) and Eq. (10) of the main text, is obtained by solving the hierarchy of coupled Schrödinger equations

$$\partial_t \Psi_n^{(\vec{k})}(t) = -i \sum_m (H_{nm}^{ex} + \delta_{nm} k_n (\omega_{\text{vib}} - i\gamma)) \Psi_m^{(\vec{k})}(t) + k_n S \omega_{\text{vib}}^2 \Psi_m^{(\vec{k}-\vec{e}_n)}(t) - \Psi_m^{(\vec{k}+\vec{e}_n)}(t), \quad (\text{S1})$$

Here,  $n$  represent the monomer indices, and  $\vec{k}$  labels different orders of the hierarchy. The superscript  $\mathbf{k} = \{k_1, k_2\}$  consists of a set of non-negative integer indices, and  $\mathbf{e}_1 = \{1, 0\}$  and  $\mathbf{e}_2 = \{0, 1\}$ . The initial conditions are  $\psi_{t=0}^{(\mathbf{0})} = \psi_{\text{ini}}$  and  $\psi_{t=0}^{(\mathbf{k})} = 0$  for  $\mathbf{k} \neq \mathbf{0}$ . The wavefunctions entering Eq. (11) of the main text are  $\phi_n(t) = \psi^{(\mathbf{0})}(t)$  with  $\psi_{\text{ini}} = |n\rangle$ , where  $n = 1, 2$ . For further details about the formalism see Ref. [2]. We use the 'triangular truncation scheme' (see e.g. Ref. [3]) with a hierarchy depth of 20. The trajectories were propagated for 3000 fs with a time step of 1 fs. We have used the HOPS implementation of D. Bennett [4].

### S II. M-LOOP PROCEDURE

We used the GPR optimizer in the M-LOOP package [5, 6]. M-LOOP performs an appropriate combination of differential evolution (DE) and GPR. The numerical routine of M-LOOP proceeds as follows:

1. DE starts from an initial parameter set (default: random) and suggests  $N$  (default:  $\max(10, 2 \times N_{\text{par}})$ ) parameter sets, which  $N_{\text{par}}$  is the number of parameters in the parameter set.
2. GPR is initiated and fits the cost function using the known parameter sets in the cost landscape.
3. To explore the uncertain regions around the current minimum of the cost, M-LOOP calculates four parameter sets from the acquisition function, Eq. (15) of the main text, at the search points. The search points are the best point so far and  $M$  (default:  $\max(10, N_{\text{par}})$ ) random points. This gives four next parameter sets. By default, for efficiency reasons, MLOOP performs at least one DE calculation between GPR ones. For our data, we realized that using only GPR calculations leads to a faster landscape convergence. That is what we used in this paper.
4. This repeats until the halting condition (for our case 1000 runs) is met.

---

\* farhadtg@pks.mpg.de

† fzhenq@uni-bremen.de

‡ eisfeld@pks.mpg.de

### S III. EXACT COST-LANDSCAPES, DIFFERENCE TO ESTIMATED ONES, AND ESTIMATED UNCERTAINTY FOR THE EXPERIMENTS DISCUSSED IN THE MAIN TEXT

Here we provide the exact landscapes of the monomer and dimers of the experiment of Ref. [7]. The 2D cross sections are extracted from the full cost function, constructed by 50 calculations for each parameter of monomer ( $50^5$  calculations in total) and 100 calculations for each parameter of dimer ( $100^4$  calculations in total). We choose the common points to be the minimum points of the full cost function.

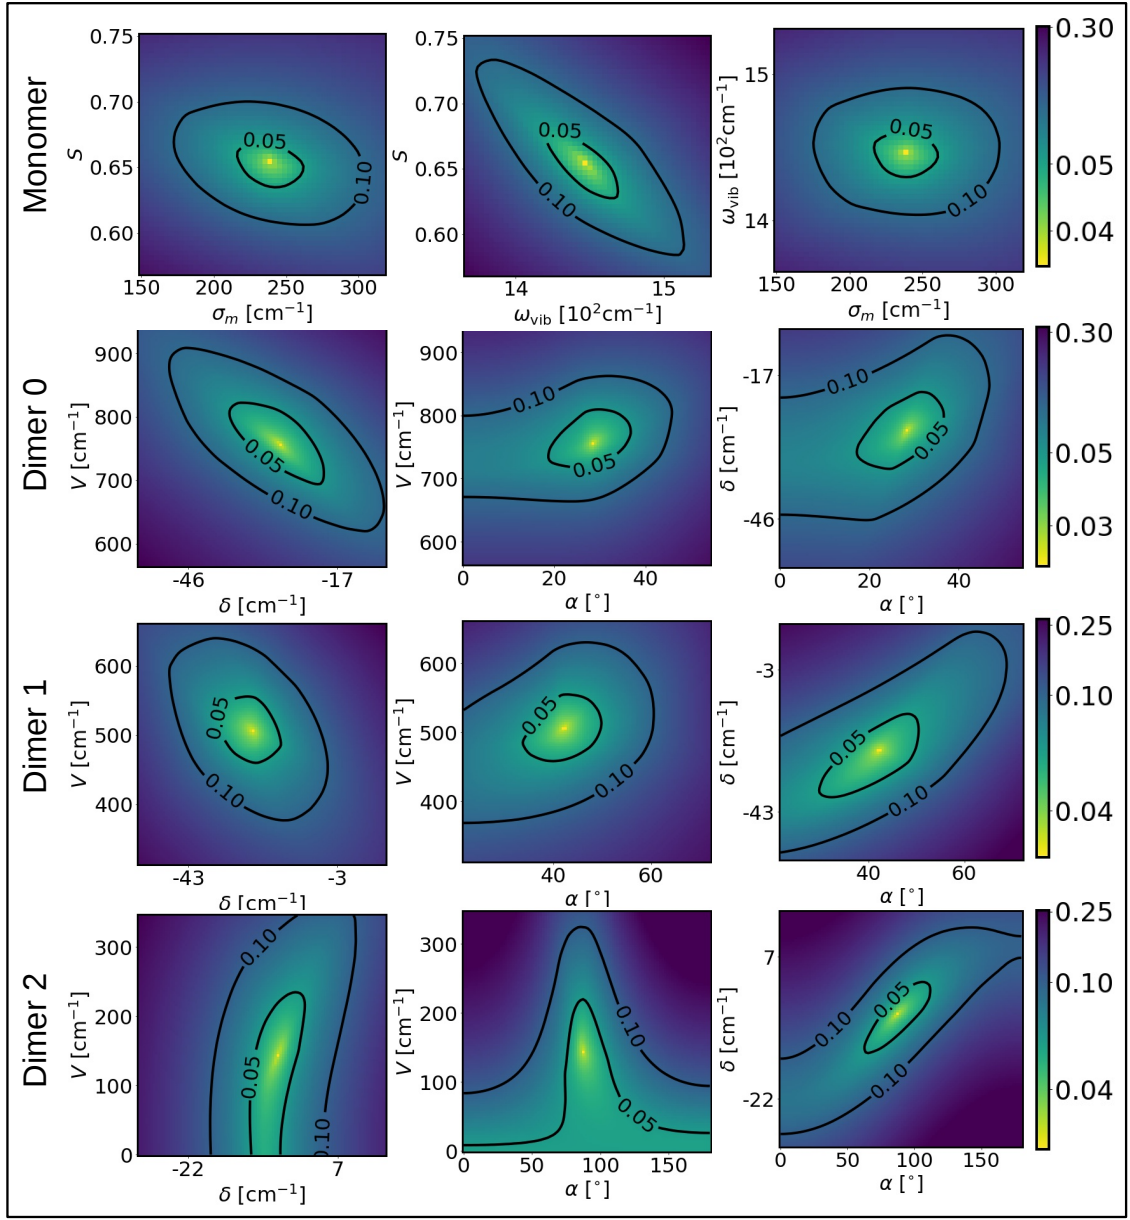

FIG. S1. The exact cost landscapes of the monomer and dimers of the experiment of Ref. [7].

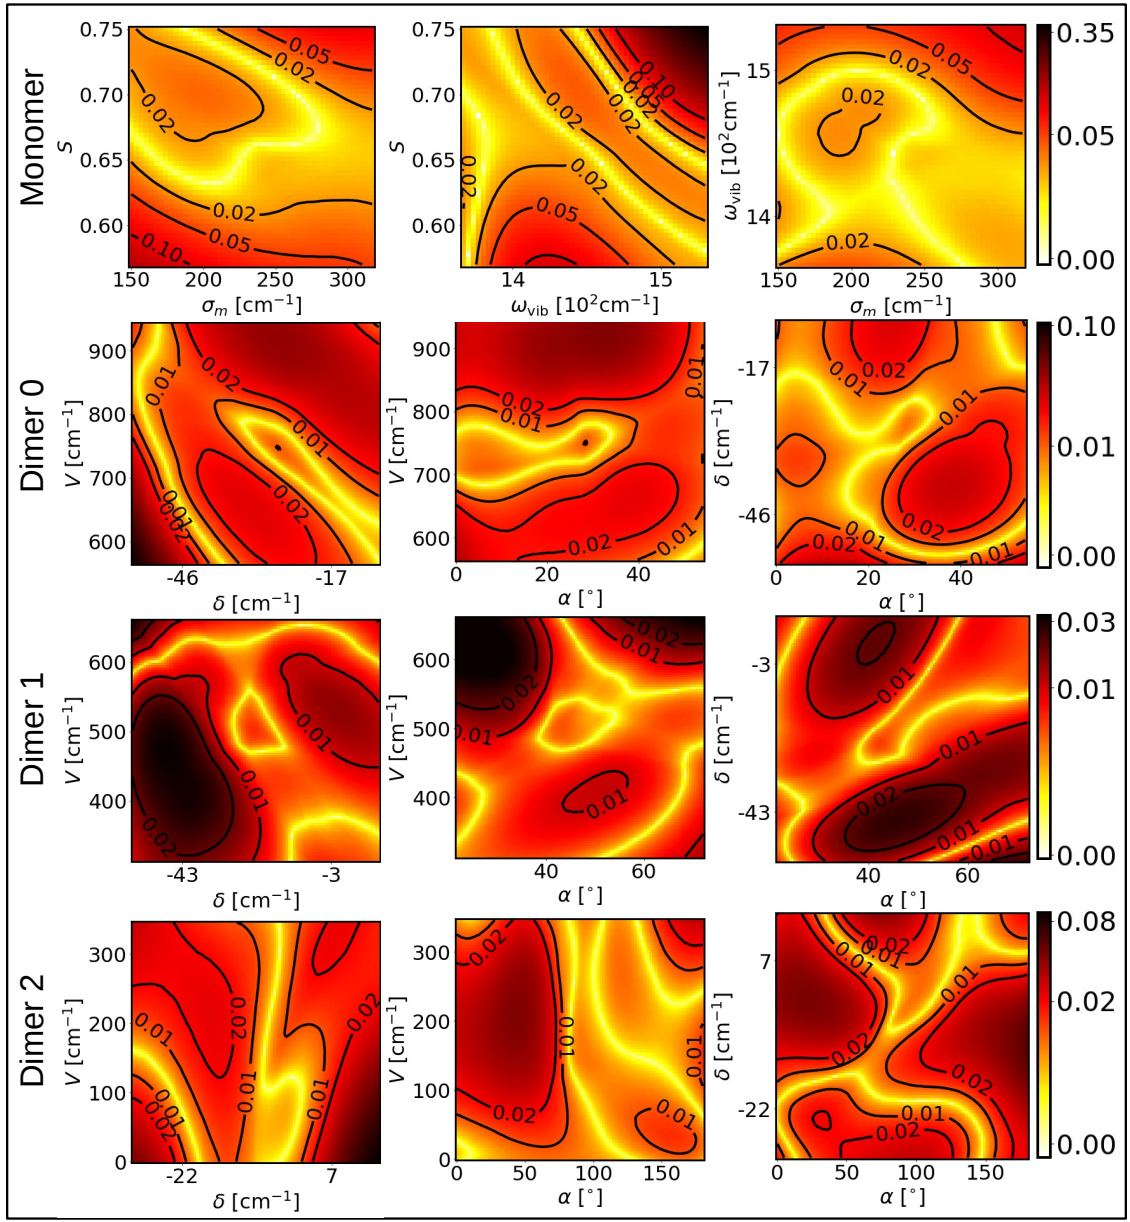

FIG. S2. The absolute difference between exact and GPR landscapes of the monomer and dimers of the experiment of Ref. [7].

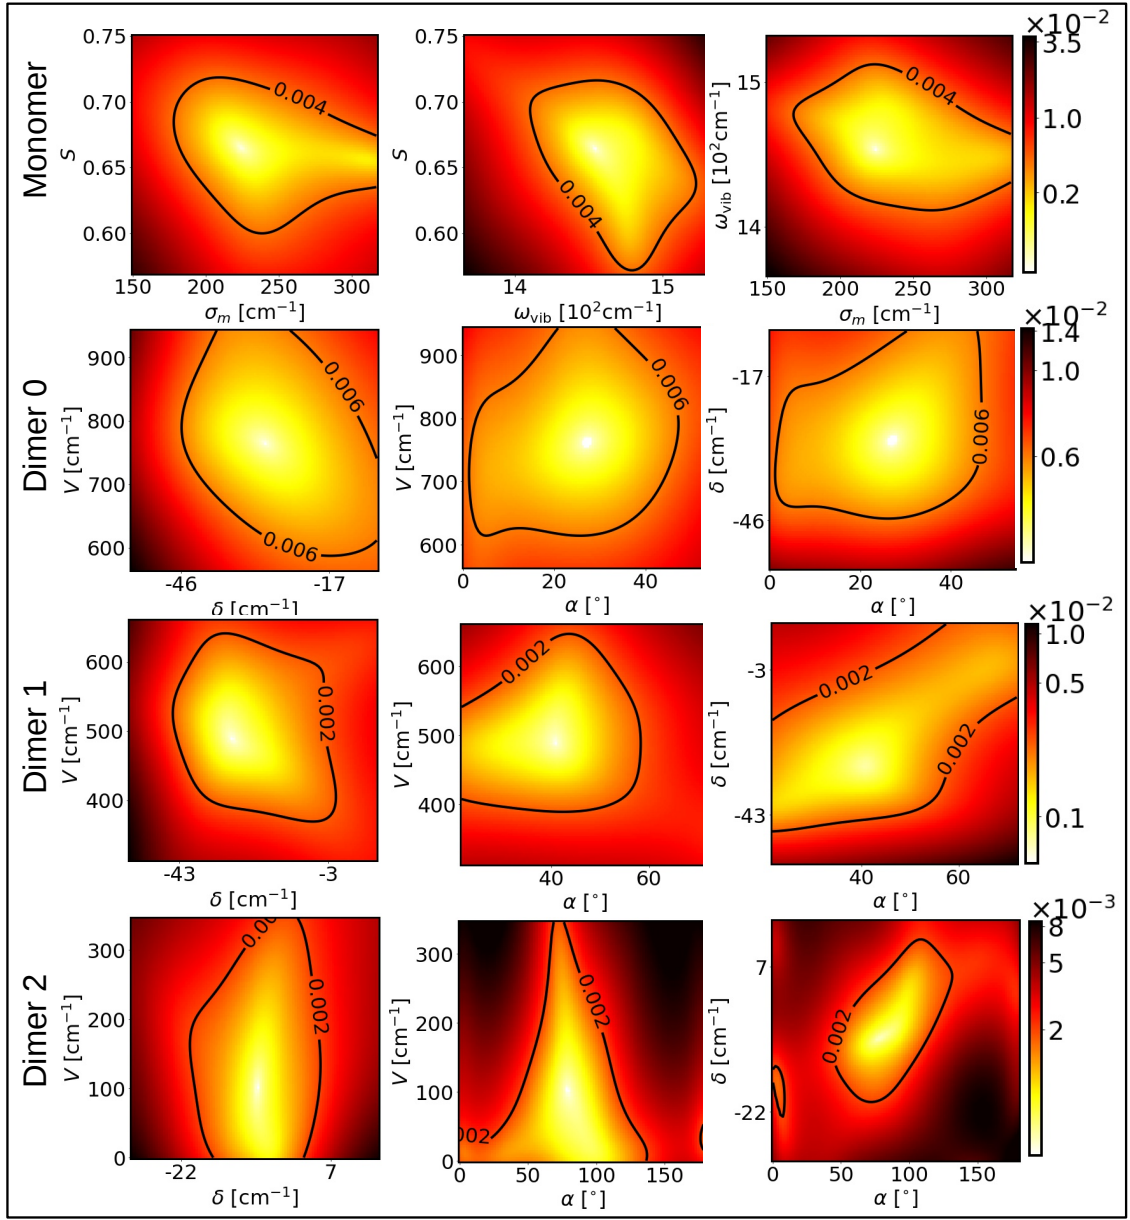

FIG. S3. The uncertainty of GPR landscapes of the monomer and dimers of the experiment of Ref. [7].

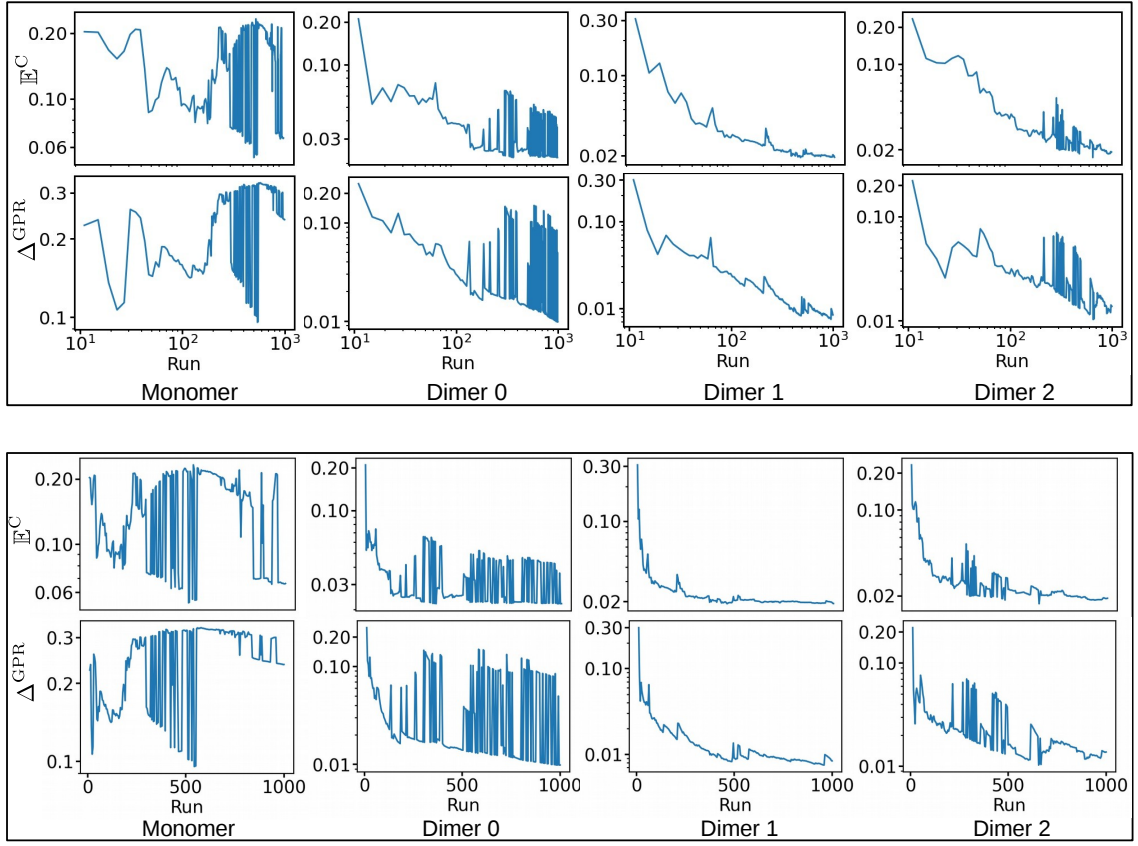

FIG. S4. The average cost  $\mathbb{E}^C$  and the average uncertainty  $\Delta^{\text{GPR}}$  of the monomer and dimers of the experiment of Ref. [7]. Top: logarithmic abscissa. Bottom: linear abscissa.

#### S IV. ESTIMATING THE ANGLE $\alpha$ FROM THE MOLECULAR STRUCTURES

To compare to the predictions of the GPR, we also estimate the angle  $\alpha$  between the monomeric transition dipoles directly using the molecular structures of the dimers reported in Ref. [7]. These structures are shown in Fig. S5.

We first note that from the DFTB+ calculations of the optimized TDI monomer, the direction of the transition dipole vector of the TDI monomer is along the direction connecting the two N atoms (blue dots in Fig. S5). Within the dimers, for each TDI monomer, the direction of the transition dipole moment is taken as the vector between these two nitrogen atoms. Finally, the angle  $\alpha$  between the two transition dipoles of the TDI monomers in the dimer is calculated as the angle between the two vectors.

As shown in Tab. III of the main text, the estimated angles between are  $9^\circ$ ,  $12^\circ$ , and  $11^\circ$  for the dimer 0, dimer 1 and dimer 2, respectively. We note that similar angles are obtained when the transition dipole moment direction is estimated using another pairs of atoms, i.e., the nitrogen and a carbon atom in the last ring of the molecule.

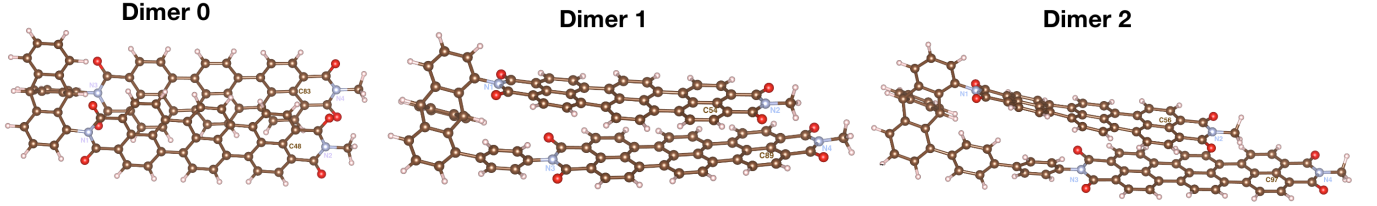

FIG. S5. Molecular structures of the dimers using the atomic coordinates given in Ref. [7]. The coordinates of the labeled atoms are used to estimate the angles between the transition dipole moments of the monomers.

## S V. MORE EXAMPLES

## A. Monomer and Dimer spectra of Ref. [8]

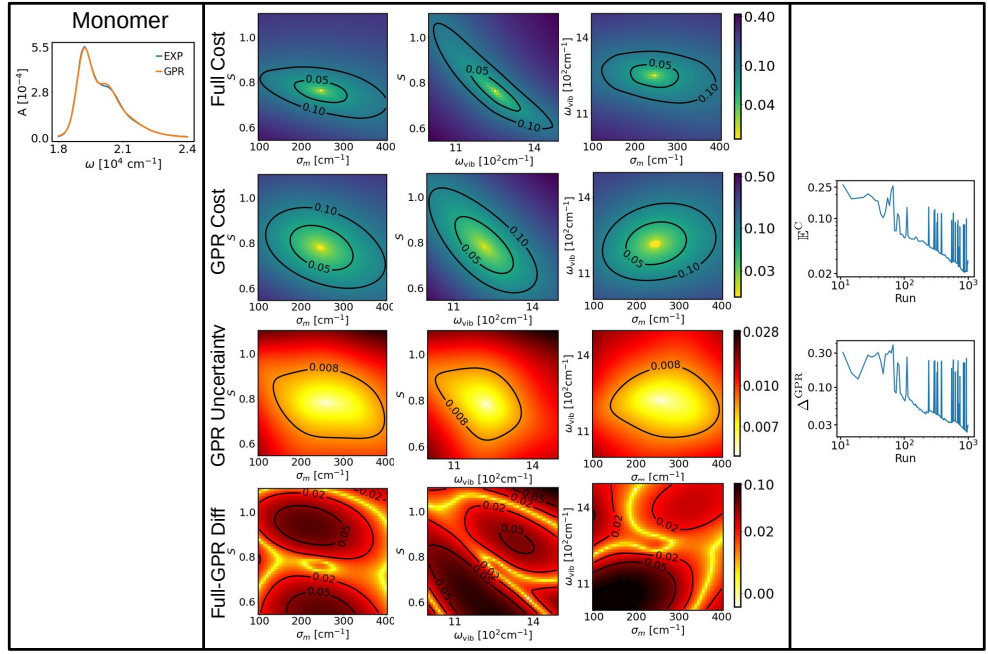

FIG. S6. The results for the monomer of the experiment of Ref. [8]. The optimal parameter set is  $\mathcal{P}_{\text{mon}}^{\text{GPR}} = [\varepsilon_e, \omega_{\text{vib}}, S, \gamma, \sigma_m] = [20004 \text{ cm}^{-1}, 1189 \text{ cm}^{-1}, 0.78, 43 \text{ cm}^{-1}, 255 \text{ cm}^{-1}]$ .

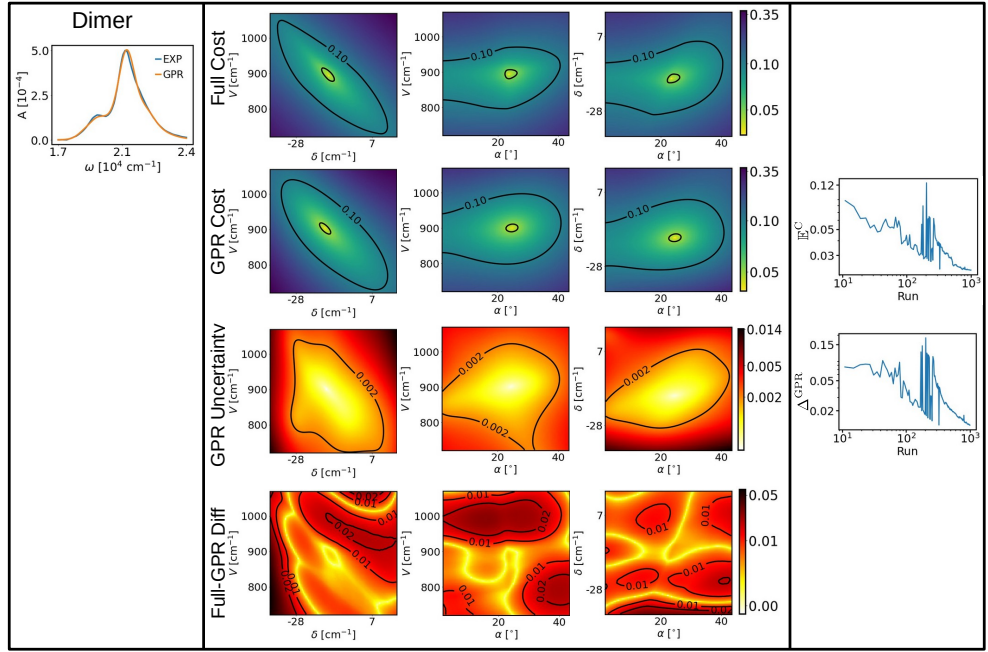

FIG. S7. The results for the dimer of the experiment of Ref. [8]. The monomer parameters given in the previous figure have been used.

### B. Monomer and Dimer spectra of Ref. [9]

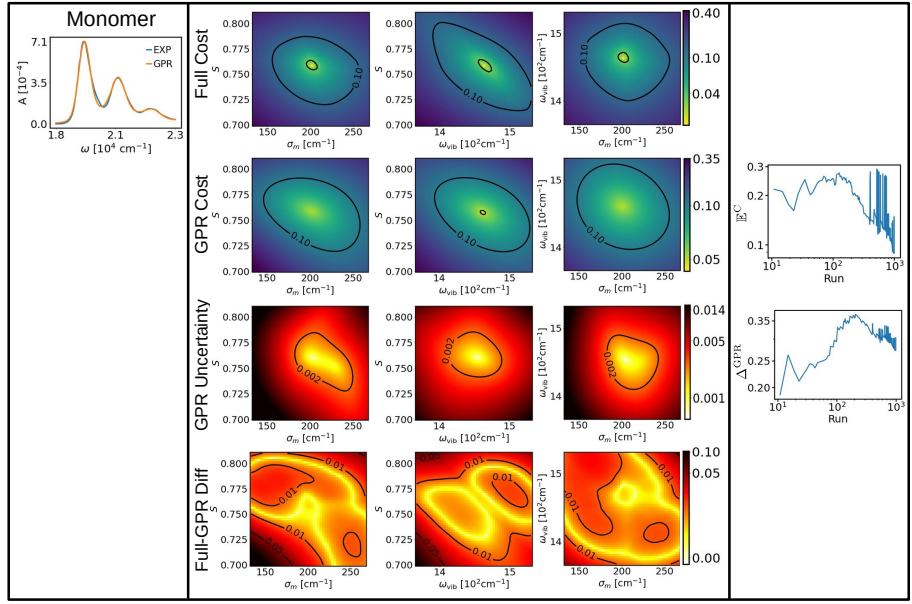

FIG. S8. The results for the monomer of the experiment of Ref. [9]. The optimal parameter set is  $\mathcal{P}_{\text{mon}}^{\text{GPR}} = [\varepsilon_e, \omega_{\text{vib}}, S, \gamma, \sigma_m] = [20263 \text{ cm}^{-1}, 1453 \text{ cm}^{-1}, 0.76, 21 \text{ cm}^{-1}, 203 \text{ cm}^{-1}]$ .

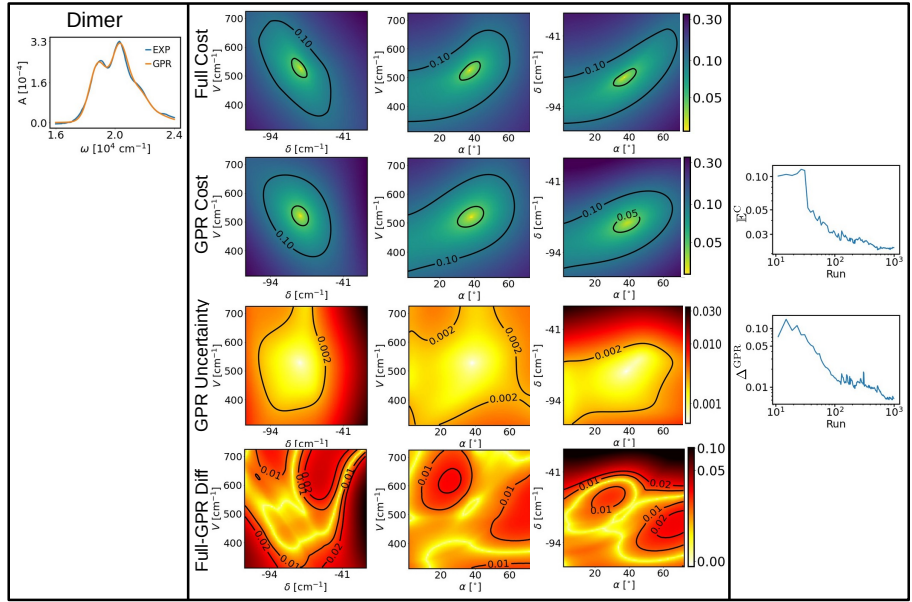

FIG. S9. The results for the dimer of the experiment of Ref. [9]. The monomer parameters given in the previous figure have been used.

- 
- [1] D. Suess, A. Eisfeld, and W. Strunz, *Physical Review Letters* **113**, 150403 (2014).
  - [2] G. Ritschel, D. Suess, S. Möbius, W. T. Strunz, and A. Eisfeld, *Journal of Chemical Physics* **142**, 034115 (2015).
  - [3] P.-P. Zhang, C. Bentley, and A. Eisfeld, *The Journal of chemical physics* **148**, 134103 (2018).
  - [4] D. Bennett, “mesohops,” <https://github.com/MesosienceLab/mesohops>.
  - [5] P. B. Wigley, P. J. Everitt, A. van den Hengel, J. W. Bastian, M. A. Sooriyabandara, G. D. McDonald, K. S. Hardman, C. D. Quinlivan, P. Manju, C. C. Kuhn, *et al.*, *Scientific Reports* **6**, 1 (2016).
  - [6] MLOOP source code and documentation found at <https://m-loop.readthedocs.io/en/stable/api/mloop.html>.
  - [7] E. A. Margulies, C. E. Miller, Y. Wu, L. Ma, G. C. Schatz, R. M. Young, and M. R. Wasielewski, *Nature Chemistry* **8**, 1120 (2016).
  - [8] I. Baraldi, M. Caselli, F. Momicchioli, G. Ponterini, and D. Vanossi, *Chemical physics* **275**, 149 (2002).
  - [9] M. Son, K. H. Park, C. Shao, F. Würthner, and D. Kim, *The journal of physical chemistry letters* **5**, 3601 (2014).
